# Supplementary material for: A Metric Learning Reality Check
Source: arXiv:2003.08505 source file (2020-09-16)
Supplement: Supplementary file 1 [file supplementary.tex]

\section*{Additional results}

Table \ref{CUB200ResultsBatchSize256} shows results on CUB200 with a batch size of 256 instead of 32. The increase in batch size gives FastAP a significant boost in accuracy, and as a result, it performs on par with the rest of the methods, rather than underperforming. See \href{https://www.github.com/KevinMusgrave/powerful-benchmarker}{github.com/KevinMusgrave/powerful-benchmarker} for more supplementary material, including the source code, configuration files, log files, and interactive bayesian optimization plots. 

\bgroup

\begin{table}[]
\begin{center}
\caption{Accuracy on CUB200, batch size 256}
\label{CUB200ResultsBatchSize256}
\resizebox{\textwidth}{!}{
\begin{tabular}{c|ccc|ccc}
          & \multicolumn{3}{c|}{\textbf{Concatenated (512-dim)}}  & \multicolumn{3}{c}{\textbf{Separated (128-dim)}}  \\ \hline
                 & \textbf{P@1} & \textbf{RP} & \textbf{MAP@R}   & \textbf{P@1} & \textbf{RP} & \textbf{MAP@R} \\ \hline
        Pretrained & 51.05 & 24.85 & 14.21 & 50.54 & 25.12 & 14.53 \\ \hline
        Contrastive & $67.60 \pm 0.40$ & $37.08 \pm 0.14$ & $26.25 \pm 0.16$ & $59.61 \pm 0.18$ & $31.85 \pm 0.10$ & $21.03 \pm 0.10$  \\ \hline
        Triplet & $63.92 \pm 0.32$ & $34.32 \pm 0.39$ & $23.51 \pm 0.38$ & $56.08 \pm 0.23$ &	$29.82 \pm 0.25$ & $19.02 \pm 0.23$ \\ \hline
        NTXent & $66.88 \pm 0.36$ & $37.04 \pm 0.16$ & $26.13 \pm 0.18$ & $59.38 \pm 0.14$ & $32.14 \pm 0.12$ & $21.18 \pm 0.12$ \\ \hline
        ProxyNCA & $66.21 \pm 0.30$ & $36.38 \pm 0.12$ & $25.53 \pm 0.13$ & $58.83 \pm 0.24$ & $31.60 \pm 0.15$ & $20.76 \pm 0.16$ \\ \hline
        Margin & $64.98 \pm 0.43$ & $35.15 \pm 0.29$ & $24.13 \pm 0.28$ & $56.38 \pm 0.42$ & $29.76 \pm 0.22$ & $18.81 \pm 0.20$ \\ \hline 
        Margin / class & $66.51 \pm 0.42$ &	$36.11 \pm 0.19$ & $25.18 \pm 0.19$ & $58.29 \pm 0.32$ & $31.03 \pm 0.18$ & $20.04 \pm 0.17$ \\ \hline
        N. Softmax & $66.18 \pm 0.41$ & $36.15 \pm 0.22$ & $25.33 \pm 0.23$ & $59.08 \pm 0.30$ & $31.78 \pm 0.18$ & $20.95 \pm 0.18$  \\ \hline
        CosFace & $66.73 \pm 0.31$ & $37.07 \pm 0.16$ &	$26.23 \pm 0.18$ & $59.82 \pm 0.22$ &	$32.06 \pm 0.11$ & $21.24 \pm 0.11$ \\ \hline
        ArcFace & $66.61 \pm 0.44$ & $36.94 \pm 0.24$ & $26.08 \pm 0.25$ & $60.08 \pm 0.30$ & $32.46 \pm 0.16$ & $21.60 \pm 0.15$ \\ \hline
        FastAP & $66.54 \pm 0.47$ & $37.07 \pm 0.23$ & $26.18 \pm 0.24$ & $59.26 \pm 0.25$ & $32.23 \pm 0.18$ & $21.32 \pm 0.17$ \\ \hline
        SNR & $67.20 \pm 0.30$ & $37.38 \pm 0.13$ & $26.59 \pm 0.13$ & $59.71 \pm 0.25$ & $32.24 \pm 0.17$ & $21.43 \pm 0.15$ \\ \hline
        MS & $68.00 \pm 0.18$ & $37.66 \pm 0.13$ & $26.86 \pm 0.14$ & $\textbf{60.48} \pm \textbf{0.13}$ & $\textbf{32.83} \pm \textbf{0.08}$ & $\textbf{21.94} \pm \textbf{0.09}$ \\ \hline
        MS+Miner & $\textbf{68.52} \pm \textbf{0.37}$ & $\textbf{37.95} \pm \textbf{0.17}$ & $\textbf{27.08} \pm \textbf{0.19}$ & $60.41 \pm 0.37$ & $32.61 \pm 0.15$ & $21.66 \pm 0.15$ \\ \hline
        SoftTriple & $66.74 \pm 0.38$ & $37.06 \pm 0.22$ & $26.26 \pm 0.23$ & $59.94 \pm 0.26$ & $32.21 \pm 0.11$ & $21.45 \pm 0.11$ \\ \hline

\end{tabular}}
\end{center}
\end{table}
\egroup
